# Supplementary material for: Large Language Model Critics for Execution-Free Evaluation of Code Changes
Source: arXiv:2501.16655 source file (2025-01-28)
Supplement: Supplementary file 1 [file prompts.tex]

\newpage
\section{LLM Prompts}
\label{sec:prompts}

\subsubsection{Scoring with no aggregation}
\begin{promptexample}
You are a code analysis assistant specializing in predicting test outcomes. 
You are provided with a set of functions/classes and associated tests and your task is to determine whether all of these tests will now pass or not.

<source>
{{source}}
</source>

Here is the test files containing the relevant test functions or classes.
<tests>
{{tests}}
</tests>

Please analyze the provided code and tests for your prediction. Follow these steps:

1. Carefully review the source code, focusing on the functional aspects.
2. Examine the provided tests and their assertions.
3. Reason whether each of the assertions in the provided tests, based on the provided source code, will apply or not.
4. Make reasonable assumptions about any missing context or dependencies. Note that such assumptions should result in a relatively lower confidence about your final predictions.
5. Ignore minor syntactic issues or missing API definitions, focusing on the logic and functionality.

Provide your analysis in the following format:

<analysis>
Explain your reasoning about how the patch affects the code's behavior and how it relates to the provided tests.
Discuss any potential issues or areas of concern.
</analysis>

After your analysis, provide your final prediction:

<prediction>yes</prediction>
If you believe all tests will pass after applying the patch.

<prediction>no</prediction>
If you believe one or more tests will fail after applying the patch.
Also provide your confidence level on a scale of 1-100 in the example format: <confidence>90</confidence>

Your prediction should be based solely on the functional aspects of the code changes and their potential impact on the provided test cases.
Ignore non-functional differences such as comments, coding style, or formatting.

Respond only with the analysis, confidence and prediction tags as described above.
Do not include any other text in your response.
\end{promptexample}

\subsubsection{Scoring with test-centric aggregation}
\begin{promptexample}
You are a code analysis assistant specializing in predicting test outcomes.
You are provided with a set of functions after applying a patch and a relevant unit test and your task is to determine whether this test will now pass or not.

<source>
{{source}}
</source>

Here is the test file containing the relevant test function or class.
<test>
{{test}}
</test>

To make your prediction, follow these steps:

1. Carefully review the given source code, focusing on the functional aspects.
2. Consider the provided test cases and how they relate to the source code.
3. Reason about whether the provided test case, based on the source code, will pass or fail.
4. Ignore syntactic errors or absence of any required APIs or source code, while making the best possible assumptions in this case. Note that such assumptions should result in a relatively lower confidence about your final predictions.

Provide your analysis and prediction in the following format:

<analysis>
Explain your analysis of the source code and how they relate to the provided test cases.
Discuss any potential issues or areas of concern.
</analysis>

After your analysis, provide your final determination on whether all test cases pass.
Your determination should either be <prediction>yes</prediction> or <prediction>no</prediction>.

Also provide your confidence level on a scale of 1-100 in the example format: <confidence>90</confidence>

Remember, your prediction should be based solely on the functional aspects of the code changes and their potential impact on the provided test cases.
Ignore any non-functional differences, such as comments, coding style, or formatting.

Respond only with the analysis, confidence and prediction tags as described above.
Do not include any other text in your response.
\end{promptexample}

\subsubsection{Scoring with patch test-centric aggregation}
\begin{promptexample}
You are a code analysis assistant specializing in predicting test outcomes. You are provided with a patch and a relevant unit test and your task is to determine whether this test will now pass or not.

<patch>
{{patch}}
</patch>

Here's the test file containing the relevant test function or class.
<test>
{{test}}
</test>

To make your prediction, follow these steps:

1. Carefully review the given patch, focusing on the functional changes (lines starting with '+' or '-').
2. Consider the provided test cases and how they relate to the changes in the patch.
3. Reason about whether the provided test case, based on the changes introduced by the patch, will pass or fail.
4. Ignore syntactic errors or absence of any required APIs or source code, while making the best possible assumptions in this case. Note that such assumptions should result in a relatively lower confidence about your final predictions.

Provide your analysis and prediction in the following format:

<analysis>
Explain your analysis of the patch and how the changes relate to the provided test cases. Discuss any potential issues or areas of concern.
</analysis>

After your analysis, provide your final determination on whether all test cases will pass after applying the patch. Your determination should either be <prediction>yes</prediction> or <prediction>no</prediction>.

Also provide your confidence level on a scale of 1-100 in the example format: <confidence>90</confidence>

Remember, your prediction should be based solely on the functional aspects of the code changes in the patch and their potential impact on the provided test cases. Ignore any non-functional differences, such as comments, coding style, or formatting.

Respond only with the analysis, confidence and prediction tags as described above. Do not include any other text in your response.
\end{promptexample}

\subsubsection{Scoring with patch level and no aggregation}
\begin{promptexample}
You are a code analysis assistant specializing in predicting test outcomes.
You are provided with a patch and associated tests and your task is to determine whether all of these tests will now pass or not.

<patch>
{{patch}}
</patch>

Here is the test file containing the relevant test functions or classes.
<tests>
{{tests}}
</tests>

To make your prediction, follow these steps:

1. Carefully review the given patch, focusing on the functional changes (lines starting with '+' or '-').
2. Consider the provided test cases and how they relate to the changes in the patch.
3. Reason about whether the provided test case, based on the changes introduced by the patch, will pass or fail.
4. Ignore syntactic errors or absence of any required APIs or source code, while making the best possible assumptions in this case. Note that such assumptions should result in a relatively lower confidence about your final predictions.

Provide your analysis and prediction in the following format:

<analysis>
Explain your analysis of the patch and how the changes relate to the provided test cases. Discuss any potential issues or areas of concern.
</analysis>

After your analysis, provide your final determination on whether all test cases will pass after applying the patch.
Your determination should either be <prediction>yes</prediction> or <prediction>no</prediction>.

Also provide your confidence level on a scale of 1-100 in the example format: <confidence>90</confidence>

Remember, your prediction should be based solely on the functional aspects of the code changes in the patch and their potential impact on the provided test cases.
Ignore any non-functional differences, such as comments, coding style, or formatting.

Respond only with the analysis, confidence and prediction tags as described above.
Do not include any other text in your response.
\end{promptexample}

\subsubsection{Reference free scoring without hints}
\begin{promptexample}
You are tasked with analyzing an issue description and a corresponding patch to determine if the patch successfully resolves the described issue.
Your goal is to carefully examine the issue details and the changes proposed in the patch, then decide whether the patch adequately addresses the problem.

Here are the issue description and patch you need to analyze:
<issue_description>
{{issue_description}}
</issue_description>

<patch>
{{patch}}
</patch>

To analyze the issue and patch:

1. Carefully read the issue description to understand the problem that needs to be solved.
2. Examine the patch, focusing on the actual code changes (lines starting with '+' or '-').
3. Identify the main functional changes in the patch.
4. Compare the functional changes with the requirements outlined in the issue description.
5. Consider whether the patch fully addresses all aspects of the issue.

Provide your analysis and reasoning in the following structure:

<analysis>
1. Key points from the issue description:
[List the main problems or requirements described in the issue]

2. Functional changes in the patch:
[List the main functional changes introduced by the patch]

3. Comparison of issue requirements and patch changes:
[Explain how the changes in the patch relate to the requirements of the issue]

4. Reasoning:
[Provide your reasoning for why the patch does or does not fully resolve the issue]
</analysis>

After your analysis, provide your final determination on whether the patch resolves the described issue.
Your determination should either be <prediction>yes</prediction> or <prediction>no</prediction>.

Also provide your confidence level on a scale of 1-100 in the following format: <confidence>90</confidence>

Remember to focus on whether the patch addresses all aspects of the issue described.
Consider not only if the patch fixes the immediate problem but also if it adheres to any additional requirements or constraints mentioned in the issue description.
Base your determination on whether applying the patch would fully resolve the described issue without introducing new problems or leaving any part of the issue unaddressed.
\end{promptexample}

\subsubsection{Reference free scoring with hints}
\begin{promptexample}
You are tasked with analyzing an issue description, related hints, and corresponding patch to determine if the patch successfully resolves the described issue. 
Your goal is to carefully examine the issue details, the changes proposed in the patch, and the provided hints, then decide whether the patch adequately addresses the problem.

Here are the issue description, hints, and patch you need to analyze:

<issue_description>
{{issue_description}}
</issue_description>

<hints>
{{hints}}
</hints>

<patch>
{{patch}}
</patch>

To analyze the issue, patch, and hints:

1. Carefully read the issue description to understand the problem that needs to be solved.
2. Review the hints to gain additional context and suggested solutions.
3. Examine the patch, focusing on the actual code changes (lines starting with '+' or '-').
4. Identify the main functional changes in the patch.
5. Compare the functional changes with the requirements outlined in the issue description and any relevant suggestions from the hints.
6. Consider whether the patch fully addresses all aspects of the issue and incorporates appropriate suggestions from the hints.

Provide your analysis and reasoning in the following structure:

<analysis>
1. Key points from the issue description:
[List the main problems or requirements described in the issue]

2. Relevant suggestions from hints:
[Summarize any important suggestions or context provided in the hints]

3. Functional changes in the patch:
[List the main functional changes introduced by the patch]

4. Comparison of issue requirements, hints, and patch changes:
[Explain how the changes in the patch relate to the requirements of the issue and suggestions from the hints]

5. Reasoning:
[Provide your reasoning for why the patch does or does not fully resolve the issue, considering both the issue description and hints]
</analysis>

After your analysis, provide your final determination on whether the patch resolves the described issue.
Your determination should either be <prediction>yes</prediction> or <prediction>no</prediction>.

Also provide your confidence level on a scale of 1-100 in the following format: <confidence>90</confidence>

Remember to focus on whether the patch addresses all aspects of the issue described and incorporates relevant suggestions from the hints. 
Consider not only if the patch fixes the immediate problem but also if it adheres to any additional requirements or constraints mentioned in the issue description or suggested in the hints. 
Base your determination on whether applying the patch would fully resolve the described issue without introducing new problems or leaving any part of the issue unaddressed, while also taking into account the context and suggestions provided in the hints.
\end{promptexample}
